# Supplementary material for: Towards chemical accuracy for chemi- and physisorption with an efficient density functional
Source: arXiv:2410.11248 source file (2025-08-13)
Supplement: Supplementary file 1 [file Opt_MS_rVV10_SI.pdf]

# Supporting Information for Towards chemical accuracy for chemi- and physi-sorption with an efficient density functional

Manish Kothakonda,<sup>1</sup> Ruiqi Zhang,<sup>1</sup> Jinliang Ning,<sup>1</sup> James Furness,<sup>1</sup> Abhirup Patra,<sup>2</sup> Qing Zhao,<sup>3</sup> Jianwei Sun<sup>1\*</sup>

<sup>1</sup>Department of Physics and Engineering Physics, Tulane University, New Orleans, LA 70118, USA

<sup>2</sup>Delaware Energy Institute, University of Delaware, 221 Academy Street, Newark, Delaware 19716, United States

(Presently at Shell Technology Center, Houston, TX 77082, United States)

<sup>3</sup>Department of Chemical Engineering, Northeastern University, Boston, MA 02115

\*E-mail: jsun@tulane.edu

## Contents

|                                                                                                                                                             |      |
|-------------------------------------------------------------------------------------------------------------------------------------------------------------|------|
| 1. Section S1: Optimization of parameters and minimization of $3^{rd}$ order polynomial function .....                                                      | SI-2 |
| 2. Table S1: Absolute errors of CO adsorbed on Pt(111) with respect to $\kappa$ , b and $\beta$ .....                                                       | SI-3 |
| 4. Table S2: DFT Adsorption energies (eV) for systems constituting the CE39 dataset.....                                                                    | SI-4 |
| 5. Table S3: DFT errors adsorption energies (eV) for systems constituting the CE39 dataset. Overall error statistics (eV) are also reported at the end..... | SI-5 |
| 6. Figure S1: Comparison of errors of chemisorbed and physisorbed systems.....                                                                              | SI-6 |
| 7. Figure S2: Error statistics for (a) chemisorption and (b) physisorption (c) CE39 Full data set.....                                                      | SI-7 |
| 8. References.....                                                                                                                                          | SI-8 |

# S1. OPTIMIZATION OF PARAMETERS AND MINIMIZATION OF 3<sup>rd</sup> ORDER POLYNOMIAL FUNCTION

The standard semilocal exchange energy of spin-unpolarized density for MS<sup>1-4</sup> is defined as:

$$E_x^{\text{sl}}[n] = \int d^3\mathbf{r} n(\mathbf{r}) \varepsilon_x^{\text{unif}}(n) F_x(p, \alpha), \quad (\text{S1})$$

where,  $\varepsilon_x^{\text{unif}}(n) = -(3/4\pi^2)(3\pi^2 n)^{1/3}$  is the exchange energy per particle of a uniform electron gas (UEG),  $p = |\nabla n|^2 / [4(3\pi^2)^{2/3} n^{8/3}] = s^2$  with  $s$  to be the reduced density gradient, and  $F_x$  the enhancement factor with  $F_x = 1$  for LSDA. The equation S1 explains the separation of  $\alpha$ - and  $p$ -dependence<sup>3</sup>, in exchange enhancement factor as  $\alpha$  is vital in recognizing different orbital-overlapping regions<sup>5</sup>, where  $\alpha = 0$  is single orbital region which characterizes covalent bonding,  $\alpha \approx 1$  identifies the slowly varying density regime characterizing metallic bonding, and  $\alpha \geq 1$  is weakly overlapped region for non-covalent interactions. For MS2  $F_x(p, \alpha)$  in equation S1 is given by:

$$F_x^{\text{int}}(p, \alpha) = F_x^1(p) + f(\alpha)[F_x^0(p) - F_x^1(p)] \quad (\text{S2})$$

where,

$$F_x^1(p) = F_x^{\text{int}}(p, \alpha = 1) = 1 + \kappa - \frac{\kappa}{1 + \frac{\mu^{\text{GE}} p}{\kappa}}, \quad (\text{S3})$$

and

$$F_x^0(p) = F_x^{\text{int}}(p, \alpha = 0) = 1 + \kappa - \frac{\kappa}{1 + \frac{\mu^{\text{GE}} p + c}{\kappa}}, \quad (\text{S4})$$

is the single orbital enhancement, and

$$f(\alpha) = \frac{(1 - \alpha^2)^3}{1 + \alpha^3 + b\alpha^6}, \quad (\text{S5})$$

is a function that interpolates and extrapolates these limits. In Eq. S5 the parameter  $b$  controls the  $\alpha$  which identifies the different types of bonding regions namely, slowly varying density, metallic bonding and weak non-covalent interactions. In addition,  $b$  parameter controls the interpolation behaviour and sets the  $\alpha \rightarrow \infty$  limit. In Eqs. S3 and S4,  $\kappa$  controls the functional's density gradient response through  $s$ .

Now we discuss about the the rVV10 non-local correlation functional<sup>6</sup> which is a modification of the VV10 correlation kernel<sup>7</sup> which takes the form based on Rutgers-Chalmers vdW-DFs shown in the Eq. S6.

$$E_c^{\text{nl}} = \frac{1}{2} \int \int d\mathbf{r} n(\mathbf{r}) [d\mathbf{r}' \phi(\mathbf{r}, \mathbf{r}') n(\mathbf{r}') + \beta] \quad (\text{S6})$$

where  $n(\mathbf{r})$  is the electron density and  $\phi(\mathbf{r}, \mathbf{r}')$  is the kernel describing the density-density interactions.  $\beta$  controls short range damping of  $R^{-6}$  ( $R = |\mathbf{r} - \mathbf{r}'|$ ) asymptote. To ensure zero  $E_c^{\text{nl}}$  for the uniform electron gas,  $\beta = \frac{1}{32}(3/b_{\text{vdW}})^{\frac{3}{4}}$  in Hartrees is required for rVV10.  $b_{\text{param}}$  in the original form is changed to  $b_{\text{vdW}}$  to avoid confusion with  $b$  in mGGA-MS. The two empirical parameters  $C$  and  $b_{\text{vdW}}$  appear in the kernel:  $C = 0.0093$  is chosen for accurate  $-C_6/R^6$  vdW interaction between molecules at large separation  $R$ , and  $b_{\text{vdW}}$  which is dependent on  $\beta$  controlling the damping of  $E_c^{\text{nl}}$  is fitted to the Ar<sub>2</sub> dimer binding energy curve for each  $\kappa$  and  $b$ .

In the original form in MS2,  $b = 4.0$ , and  $\kappa = 0.504$  was determined by Averaged Mean Absolute Errors of atomization energies subset AE6, and barrier heights subset BH6 minimized by surface fitted function. Here, we combine the two parameters of MS ( $b, \kappa$ ) and one parameter of rVV10 ( $b_{\text{vdW}}$ ) fitted together to the Ar<sub>2</sub> dimer binding energies and adsorption energy of CO/Pt(111). A coarse grid in  $\kappa$  and  $b$  two dimensional fitting space is made. The  $b_{\text{vdW}}$  was re-fit for each  $(\kappa, b)$  for six points of Ar<sub>2</sub> binding curve. Then we calculate adsorption energies of CO/Pt(111) surface for each of  $(\kappa, b)$ . The absolute errors of CO/Pt(111) adsorption shown in Table S1 was fitted to 3<sup>rd</sup> order polynomial equation in  $\kappa$  and  $b$  2D space is represented in the figure 2 in the main manuscript was minimized to optimize the parameters  $\kappa = 0.2501$ ,  $b = 0.9104$  and  $\beta = 26.26$ .

TABLE S1. Absolute errors of CO adsorbed on Pt(111) with respect to  $\kappa$ , b and  $\beta$ 

| <b>Kappa (<math>\kappa</math>)</b> | <b>b</b> | <b>c</b>   | $\beta$ | <b>Absolute Error CO/Pt(111) eV</b> |
|------------------------------------|----------|------------|---------|-------------------------------------|
| 0.2                                | 0.6      | 0.8650485  | 13.6    | 0.2508110                           |
| 0.2                                | 0.8      | 0.8650485  | 24.51   | 0.2435690                           |
| 0.2                                | 1        | 0.8650485  | 72.85   | 0.2346810                           |
| 0.2                                | 1.2      | 0.8650485  | 81.46   | 0.2611830                           |
| 0.2                                | 1.44     | 0.8650485  | 288.33  | 0.2746470                           |
| 0.245                              | 0.6      | 0.41234953 | 12.63   | 0.2382290                           |
| 0.245                              | 0.8      | 0.41234953 | 20.38   | 0.2335860                           |
| 0.245                              | 1        | 0.41234953 | 37.1    | 0.2375960                           |
| 0.245                              | 1.2      | 0.41234953 | 98.84   | 0.2290010                           |
| 0.245                              | 1.44     | 0.41234953 | 138.2   | 0.2480500                           |
| 0.29                               | 0.6      | 0.28790598 | 10.72   | 0.2456092                           |
| 0.29                               | 0.8      | 0.28790598 | 15.5    | 0.2404080                           |
| 0.29                               | 1        | 0.28790598 | 21.91   | 0.2389270                           |
| 0.29                               | 1.2      | 0.28790598 | 31.8    | 0.2409970                           |
| 0.29                               | 1.44     | 0.28790598 | 60.73   | 0.2629710                           |
| 0.34                               | 0.6      | 0.22454422 | 8.91    | 0.2639880                           |
| 0.34                               | 0.8      | 0.22454422 | 12.08   | 0.2536260                           |
| 0.34                               | 1        | 0.22454422 | 15.09   | 0.2542321                           |
| 0.34                               | 1.2      | 0.22454422 | 18.7    | 0.2528130                           |
| 0.34                               | 1.44     | 0.22454422 | 23.64   | 0.2508810                           |
| 0.3928                             | 0.6      | 0.18741979 | 7.45    | 0.2926470                           |
| 0.3928                             | 0.8      | 0.18741979 | 9.47    | 0.2796840                           |
| 0.3928                             | 1        | 0.18741979 | 11.38   | 0.2746390                           |
| 0.3928                             | 1.2      | 0.18741979 | 13.2    | 0.2723210                           |
| 0.3928                             | 1.44     | 0.18741979 | 15.36   | 0.2713650                           |

TABLE S2. DFT Adsorption energies (eV) for systems constituting the CE39 dataset.

| Reaction Name       | Site   | C   | Expt  | LDA     | PBE   | RPBE  | RPBE+D3 | optPBE-vdW | BEEF+vdW | MS2   | SCAN  | SCAN+rVV10 | Opt(MS+rVV10) |
|---------------------|--------|-----|-------|---------|-------|-------|---------|------------|----------|-------|-------|------------|---------------|
| CO/Ni(111)          | fcc    | 1/4 | -1.28 | -2.7872 | -1.81 | -1.42 | -1.530  | -1.93      | -1.57    | -1.49 | -1.89 | -2.01      | -1.40         |
| CO/Pt(111)          | top    | 1/4 | -1.28 | -2.2152 | -1.64 | -1.36 | -1.770  | -1.68      | -1.39    | -1.49 | -1.94 | -2.04      | -1.52         |
| CO/Pd(111)          | fcc    | 1/4 | -1.49 | -2.7872 | -1.95 | -1.58 | -1.890  | -2.08      | -1.74    | -1.95 | -2.19 | -2.31      | -1.82         |
| CO/Pd(100)          | bridge | 1/4 | -1.63 | -2.652  | -1.86 | -1.52 | -1.840  | -1.94      | -1.61    | -1.86 | -2.09 | -2.24      | -1.90         |
| CO/Rh(111)          | top    | 1/4 | -1.47 | -2.5376 | -1.84 | -1.57 | -1.960  | -1.96      | -1.68    | -1.82 | -2.04 | -2.14      | -1.86         |
| CO/Ir(111)          | top    | 1/4 | -1.7  | -2.5376 | -1.93 | -1.67 | -2.170  | -2.03      | -1.78    | -1.84 | -2.04 | -2.14      | -1.90         |
| CO/Cu(111)          | top    | 1/4 | -0.59 | -1.3728 | -0.75 | -0.48 | -0.760  | -0.78      | -0.51    | -0.67 | -0.91 | -0.97      | -0.72         |
| CO/Ru(0001)         | top    | 1/4 | -1.67 | -2.496  | -1.88 | -1.61 | -1.930  | -1.96      | -1.71    | -1.82 | -1.95 | -2.05      | -1.92         |
| CO/Co(0001)         | top    | 1/4 | -1.23 | -2.4336 | -1.63 | -1.33 | -1.660  | -1.71      | -1.4     | -1.32 | -1.72 | -1.82      | -1.76         |
| (N+O)/Ni(100)       | hollow | 1/4 | -3.1  | -6.0112 | -4.37 | -3.72 | -3.550  | -5.27      | -3.99    | -4.27 | -4.94 | -5.1       | -3.99         |
| NO/Pt(111)          | hollow | 1/4 | -1.23 | -2.8704 | -1.83 | -1.43 | -1.900  | -2.23      | -1.52    | -1.46 | -1.91 | -2.01      | -1.28         |
| NO/Pd(111)          | fcc    | 1/4 | -1.89 | -3.276  | -2.23 | -1.83 | -2.260  | -2.8       | -2.07    | -2.18 | -2.37 | -2.48      | -1.95         |
| NO/Pd(100)          | fcc    | 1/4 | -1.69 | -3.2344 | -2.05 | -1.63 | -2.020  | -2.6       | -1.82    | -2.02 | -2.19 | -2.32      | -1.86         |
| O/Ni(111)           | hollow | 1/4 | -5.03 | -5.8864 | -4.58 | -4.08 | -4.660  | -6.12      | -4.37    | -4.48 | -5.24 | -5.34      | -5.07         |
| O/Ni(100)           | fcc    | 1/4 | -5.49 | -6.6664 | -5.07 | -4.5  | -5.110  | -6.66      | -4.92    | -5.18 | -6.19 | -6.2       | -5.65         |
| O/Pt(111)           | fcc    | 1/9 | -2.16 | -3.2552 | -2.37 | -1.86 | -2.170  | -3.2       | -2.1     | -2.43 | -2.91 | -2.94      | -1.97         |
| O/Rh(100)           | hollow | 1/4 | -3.68 | -5.7408 | -4.33 | -3.76 | -3.620  | -5.79      | -4.03    | -4.82 | -4.92 | -5.05      | -4.37         |
| H/Pt(111)           | top    | 1/4 | -0.75 | -1.664  | -0.96 | -0.65 | -0.780  | -0.79      | -0.47    | -0.86 | -1.11 | -1.12      | -0.97         |
| H/Ni(111)           | fcc    | 1/4 | -1.04 | -1.9136 | -1.1  | -0.77 | -0.970  | -1.05      | -0.69    | -1.28 | -1.28 | -1.32      | -0.92         |
| H/Ni(100)           | hollow | 1/4 | -0.9  | -1.8928 | -1.01 | -0.65 | -0.910  | -0.9       | -0.58    | -1.19 | -1.29 | -1.13      | -1.25         |
| H/Rh(111)           | fcc    | 1/4 | -0.75 | -1.872  | -1.07 | -0.76 | -0.580  | -0.91      | -0.56    | -1.2  | -1.22 | -1.25      | -1.09         |
| H/Pd(111)           | fcc    | 1/4 | -0.93 | -1.9136 | -1.2  | -0.88 | -0.950  | -1.1       | -0.73    | -1.4  | -1.44 | -1.49      | -1.27         |
| I/Pt(111)           | fcc    | 1/4 | -3.24 | -3.9104 | -2.84 | -2.27 | -2.630  | -3.28      | -2.78    | -2.99 | -3.49 | -3.81      | -2.93         |
| (CH+H+I)/Pt(111)    | fcc    | 1/4 | -4.72 | -5.4184 | -3.85 | -3.05 | -4.800  | -4.27      | -3.47    | -3.7  | -4.88 | -5.2       | -3.63         |
| (CH3+I)/Pt(111)     | top    | 1/4 | -2.17 | -2.496  | -1.66 | -1.22 | -2.250  | 2.12       | -1.68    | -1.76 | -2.36 | -2.61      | -1.77         |
| NH3/Cu(100)         | top    | 1/4 | -0.59 | -0.9048 | -0.43 | -0.21 | -0.530  | -0.6       | -0.39    | -0.46 | -0.58 | -0.69      | -0.49         |
| CH3I/Pt(111)        | fcc    | 1/4 | -0.87 | -0.7904 | -0.25 | 0     | -1.020  | -0.71      | -0.41    | -0.34 | -0.39 | -0.61      | -0.36         |
| CH3OH/Pt(111)       | top    | 1/4 | -0.57 | -0.728  | -0.21 | -0.05 | -0.500  | -0.64      | -0.34    | -0.33 | -0.73 | -0.89      | -0.33         |
| CH4/Pt(111)         | fcc    | 1/4 | -0.14 | -0.2184 | -0.02 | -0.01 | -0.220  | -0.21      | -0.15    | -0.04 | -0.08 | -0.16      | -0.10         |
| C2H6/Pt(111)        | fcc    | 1/9 | -0.28 | -0.4472 | -0.04 | -0.02 | -0.340  | -0.35      | -0.22    | -0.07 | -0.14 | -0.27      | -0.16         |
| C3H8/Pt(111)        | top    | 1/9 | -0.4  | -0.6552 | -0.05 | -0.01 | -0.470  | -0.48      | -0.3     | -0.1  | -0.2  | -0.39      | -0.24         |
| C4H10/Pt(111)       | top    | 1/9 | -0.5  | -0.8424 | -0.07 | -0.02 | -1.620  | -0.62      | -0.41    | -0.13 | -0.27 | -0.69      | -0.30         |
| C6H6/Pt(111)        | bridge | 1/9 | -1.68 | -2.756  | -0.98 | -0.17 | -1.990  | -1.8       | -0.93    | -1.59 | -1.94 | -2.48      | -1.72         |
| C6H6/Cu(111)        | fcc    | 1/9 | -0.68 | -0.8008 | -0.05 | 0     | -0.720  | -0.74      | -0.41    | -0.27 | -0.3  | -0.7       | -0.28         |
| C6H6/Ag(111)        | fcc    | 1/9 | -0.63 | -0.6344 | -0.05 | 0     | -0.570  | -0.67      | -0.32    | -0.22 | -0.27 | -0.67      | -0.35         |
| C6H6/Au(111)        | fcc    | 1/9 | -0.72 | -0.4056 | -0.05 | -0.01 | -0.690  | -0.76      | -0.41    | -0.26 | -0.38 | -0.71      | -0.39         |
| C6H10/Pt(111)       | top    | 1/9 | -1.26 | -1.8408 | -0.63 | -0.07 | -1.620  | -1.55      | -0.81    | -0.95 | -1.38 | -1.81      | -1.19         |
| H2O/Pt(111)         | top    | 1/4 | -0.57 | -0.6552 | -0.21 | -0.05 | -0.380  | -0.39      | -0.22    | -0.09 | -0.66 | -0.75      | -0.27         |
| (H2O... OH)/Pt(111) | hex    | 1/9 | -0.69 | -1.2688 | -0.66 | -0.19 | -0.870  | -1.2       | -0.61    | -0.91 | -1.13 | -1.29      | -0.75         |

TABLE S3. DFT errors adsorption energies (eV) for systems constituting the CE39 dataset. Overall error statistics (eV) are also reported at the end

| Reaction Name                            | LDA    | PBE    | RPBE   | RPBE+D3 | optPBE-vdW | BEEF+vdW | MS2    | SCAN   | SCAN+rVV10 | Opt(MS+rVV10) |
|------------------------------------------|--------|--------|--------|---------|------------|----------|--------|--------|------------|---------------|
| CO/Ni(111)                               | -1.507 | -0.530 | -0.140 | -0.250  | -0.650     | -0.290   | -0.210 | -0.610 | -0.730     | -0.12         |
| CO/Pt(111)                               | -0.935 | -0.360 | -0.080 | -0.490  | -0.400     | -0.110   | -0.210 | -0.660 | -0.760     | -0.24         |
| CO/Pd(111)                               | -1.297 | -0.460 | -0.090 | -0.400  | -0.590     | -0.250   | -0.460 | -0.700 | -0.820     | -0.33         |
| CO/Pd(100)                               | -1.022 | -0.230 | 0.110  | -0.210  | -0.310     | 0.020    | -0.230 | -0.460 | -0.610     | -0.27         |
| CO/Rh(111)                               | -1.068 | -0.370 | -0.100 | -0.490  | -0.490     | -0.210   | -0.350 | -0.570 | -0.670     | -0.39         |
| CO/Ir(111)                               | -0.838 | -0.230 | 0.030  | -0.470  | -0.330     | -0.080   | -0.140 | -0.340 | -0.440     | -0.20         |
| CO/Cu(111)                               | -0.783 | -0.160 | 0.110  | -0.170  | -0.190     | 0.080    | -0.080 | -0.320 | -0.380     | -0.13         |
| CO/Ru(0001)                              | -0.826 | -0.210 | 0.060  | -0.260  | -0.290     | -0.040   | -0.150 | -0.280 | -0.380     | -0.25         |
| CO/Co(0001)                              | -1.204 | -0.400 | -0.100 | -0.430  | -0.480     | -0.170   | -0.090 | -0.490 | -0.590     | -0.53         |
| (N+O)/Ni(100)                            | -2.911 | -1.270 | -0.620 | -0.450  | -2.170     | -0.890   | -1.170 | -1.840 | -2.000     | -0.89         |
| NO/Pt(111)                               | -1.640 | -0.600 | -0.200 | -0.670  | -1.000     | -0.290   | -0.230 | -0.680 | -0.780     | -0.05         |
| NO/Pd(111)                               | -1.386 | -0.340 | 0.060  | -0.370  | -0.910     | -0.180   | -0.290 | -0.480 | -0.590     | -0.06         |
| NO/Pd(100)                               | -1.544 | -0.360 | 0.060  | -0.330  | -0.910     | -0.130   | -0.330 | -0.500 | -0.630     | -0.17         |
| O/Ni(111)                                | -0.856 | 0.450  | 0.950  | 0.370   | -1.090     | 0.660    | 0.550  | -0.210 | -0.310     | -0.04         |
| O/Ni(100)                                | -1.176 | 0.420  | 0.990  | 0.380   | -1.170     | 0.570    | 0.310  | -0.700 | -0.710     | -0.16         |
| O/Pt(111)                                | -1.095 | -0.210 | 0.300  | -0.010  | -1.040     | 0.060    | -0.270 | -0.750 | -0.780     | 0.19          |
| O/Rh(100)                                | -2.061 | -0.650 | -0.080 | 0.060   | -2.110     | -0.350   | -1.140 | -1.240 | -1.370     | -0.69         |
| H/Pt(111)                                | -0.914 | -0.210 | 0.100  | -0.030  | -0.040     | 0.280    | -0.110 | -0.360 | -0.370     | -0.22         |
| H/Ni(111)                                | -0.874 | -0.060 | 0.270  | 0.070   | -0.010     | 0.350    | -0.240 | -0.240 | -0.280     | 0.12          |
| H/Ni(100)                                | -0.993 | -0.110 | 0.250  | -0.010  | 0.000      | 0.320    | -0.290 | -0.390 | -0.230     | -0.35         |
| H/Rh(111)                                | -1.122 | -0.320 | -0.010 | 0.170   | -0.160     | 0.190    | -0.450 | -0.470 | -0.500     | -0.34         |
| H/Pd(111)                                | -0.984 | -0.270 | 0.050  | -0.020  | -0.170     | 0.200    | -0.470 | -0.510 | -0.560     | -0.34         |
| I/Pt(111)                                | -0.670 | 0.400  | 0.970  | 0.610   | -0.040     | 0.460    | 0.250  | -0.250 | -0.570     | 0.31          |
| (CH+H+I)/Pt(111)                         | -0.698 | 0.870  | 1.670  | -0.080  | 0.450      | 1.250    | 1.020  | -0.160 | -0.480     | 1.09          |
| (CH3+I)/Pt(111)                          | -0.326 | 0.510  | 0.950  | -0.080  | 4.290      | 0.490    | 0.410  | -0.190 | -0.440     | 0.40          |
| NH3/Cu(100)                              | -0.315 | 0.160  | 0.380  | 0.060   | -0.010     | 0.200    | 0.130  | 0.010  | -0.100     | 0.10          |
| CH3I/Pt(111)                             | 0.080  | 0.620  | 0.870  | -0.150  | 0.160      | 0.460    | 0.530  | 0.480  | 0.260      | 0.51          |
| CH3OH/Pt(111)                            | -0.158 | 0.360  | 0.520  | 0.070   | -0.070     | 0.230    | 0.240  | -0.160 | -0.320     | 0.24          |
| CH4/Pt(111)                              | -0.078 | 0.120  | 0.130  | -0.080  | -0.070     | -0.010   | 0.100  | 0.060  | -0.020     | 0.04          |
| C2H6/Pt(111)                             | -0.167 | 0.240  | 0.260  | -0.060  | -0.070     | 0.060    | 0.210  | 0.140  | 0.010      | 0.12          |
| C3H8/Pt(111)                             | -0.255 | 0.350  | 0.390  | -0.070  | -0.080     | 0.100    | 0.300  | 0.200  | 0.010      | 0.16          |
| C4H10/Pt(111)                            | -0.342 | 0.430  | 0.480  | -1.120  | -0.120     | 0.090    | 0.370  | 0.230  | -0.190     | 0.20          |
| C6H6/Pt(111)                             | -1.076 | 0.700  | 1.510  | -0.310  | -0.120     | 0.750    | 0.090  | -0.260 | -0.800     | -0.04         |
| C6H6/Cu(111)                             | -0.121 | 0.630  | 0.680  | -0.040  | -0.060     | 0.270    | 0.410  | 0.380  | -0.020     | 0.40          |
| C6H6/Ag(111)                             | -0.004 | 0.580  | 0.630  | 0.060   | -0.040     | 0.310    | 0.410  | 0.360  | -0.040     | 0.28          |
| C6H6/Au(111)                             | 0.314  | 0.670  | 0.710  | 0.030   | -0.040     | 0.310    | 0.460  | 0.340  | 0.010      | 0.33          |
| C6H10/Pt(111)                            | -0.581 | 0.630  | 1.190  | -0.360  | -0.290     | 0.450    | 0.310  | -0.120 | -0.550     | 0.07          |
| H2O/Pt(111)                              | -0.085 | 0.360  | 0.520  | 0.190   | 0.180      | 0.350    | 0.480  | -0.090 | -0.180     | 0.30          |
| (H2O...OH)/Pt111                         | -0.579 | 0.030  | 0.500  | -0.180  | -0.510     | 0.080    | -0.220 | -0.440 | -0.600     | -0.06         |
| Mean signed deviation (MSD)              | -0.823 | 0.030  | 0.366  | -0.142  | -0.281     | 0.143    | -0.014 | -0.315 | -0.475     | -0.026        |
| Mean absolute deviation (MAD)            | 0.843  | 0.407  | 0.439  | 0.243   | 0.541      | 0.297    | 0.352  | 0.427  | 0.489      | 0.275         |
| Root mean square deviation (RMSD)(All)   | 1.033  | 0.472  | 0.610  | 0.338   | 0.965      | 0.390    | 0.434  | 0.539  | 0.620      | 0.353         |
| Root mean square deviation (RMSD)(1-25)  | 0.956  | 0.318  | 0.236  | 0.295   | 0.699      | 0.210    | 0.271  | 0.449  | 0.526      | 0.238         |
| Root mean square deviation (RMSD)(26-39) | 0.382  | 0.472  | 0.709  | 0.336   | 0.137      | 0.325    | 0.331  | 0.254  | 0.303      | 0.248         |
| Root mean square deviation (RMSD)(1-9)   | 1.077  | 0.348  | 0.095  | 0.372   | 0.437      | 0.165    | 0.243  | 0.513  | 0.617      | 0.298         |
| Root mean square deviation (RMSD)(10-13) | 1.510  | 0.502  | 0.189  | 0.432   | 0.979      | 0.288    | 0.383  | 0.669  | 0.767      | 0.241         |
| Root mean square deviation (RMSD)(14-22) | 0.586  | 0.173  | 0.243  | 0.094   | 0.476      | 0.188    | 0.255  | 0.310  | 0.330      | 0.162         |
| Root mean square deviation (RMSD)(14-22) | 0.238  | 0.225  | 0.460  | 0.178   | 1.240      | 0.265    | 0.202  | 0.094  | 0.219      | 0.214         |

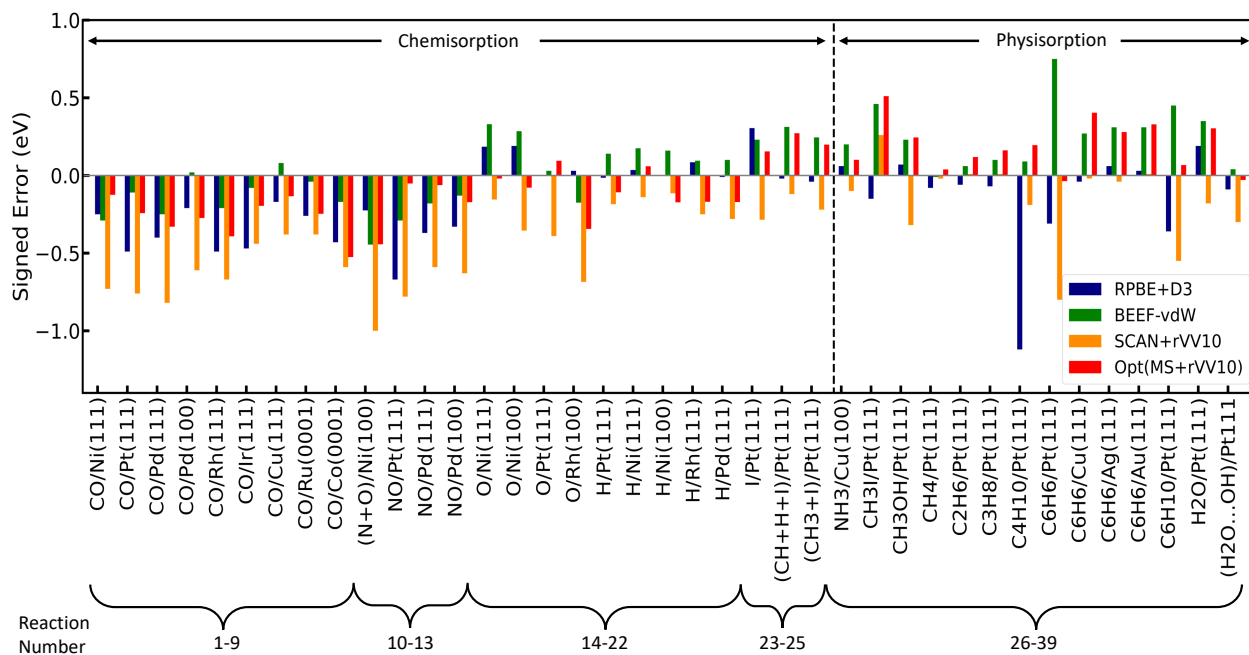

FIG. S1. Comparison of errors of chemisorbed and physisorbed systems using RPBE+D3<sup>8</sup>, BEEF-vdW<sup>9,10</sup>, SCAN+rVV10<sup>11</sup> and OptMS+rVV10. The systems right of the dashed black line are physisorbed, and left of the dashed line are dominated by covalent bonding. All errors are scaled by the number of adsorbates.

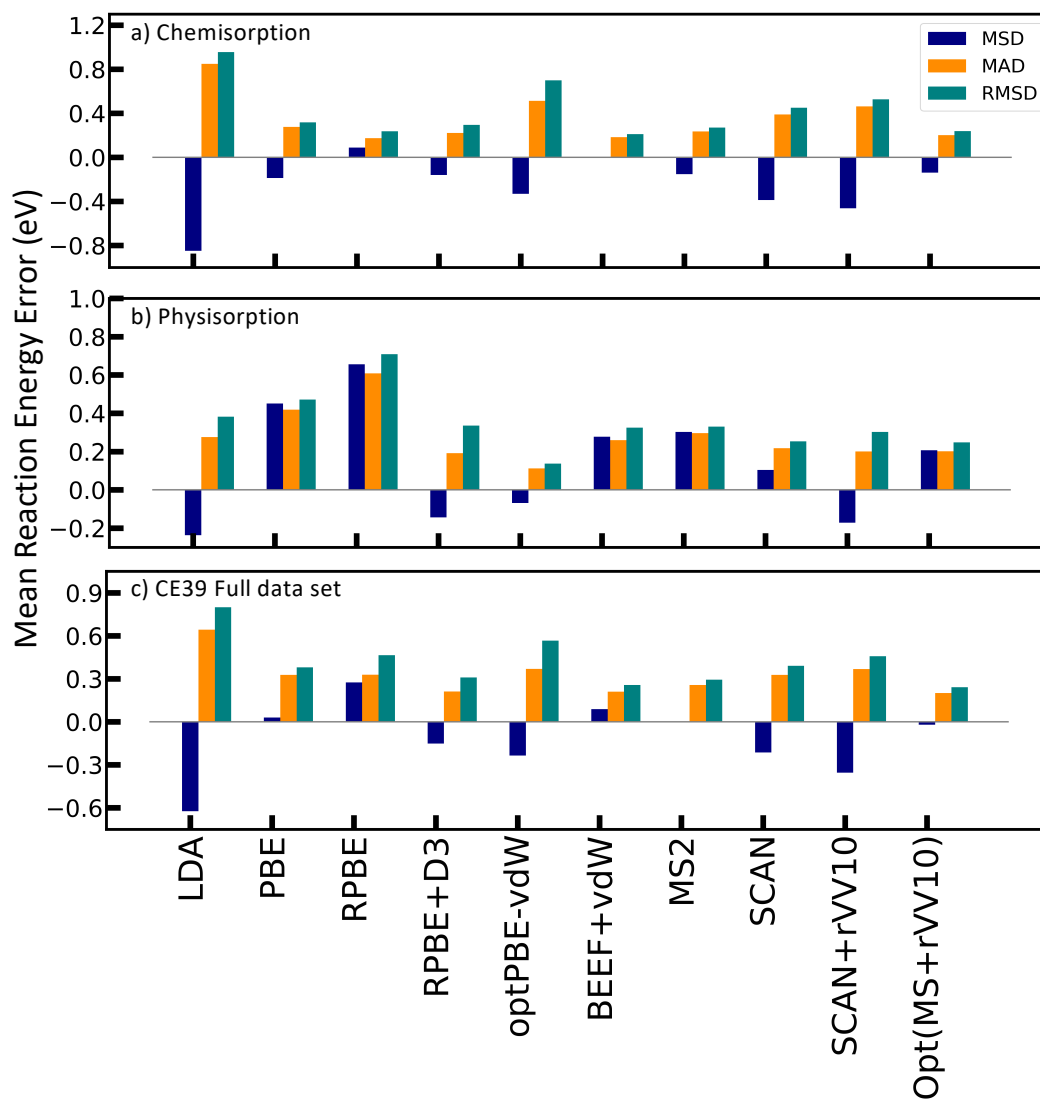

FIG. S2. Error statistics for (a) chemisorption and (b) physisorption (c) CE39 Full data set energies of PBE<sup>9</sup>, RPBE<sup>9</sup>, RPBE+D3<sup>8</sup>, optPBE-vdW<sup>12</sup>, BEEF-vdW<sup>9,10</sup>, MS2, SCAN, SCAN+rVV10 and Opt(MS+rVV10) functionals with the VASP code<sup>13-15</sup>

- 
- <sup>1</sup> J. Sun, B. Xiao, and A. Ruzsinszky, *The Journal of Chemical Physics* **137**, 051101 (2012).
- <sup>2</sup> J. Sun, R. Haunschild, B. Xiao, I. W. Bulik, G. E. Scuseria, and J. P. Perdew, *The Journal of chemical physics* **138**, 044113 (2013).
- <sup>3</sup> J. P. Perdew and Y. Wang, *Phys. Rev. B* **45**, 13244 (1992).
- <sup>4</sup> J. Sun, J. P. Perdew, and M. Seidl, *Phys. Rev. B* **81**, 085123 (2010).
- <sup>5</sup> J. Sun, B. Xiao, Y. Fang, R. Haunschild, P. Hao, A. Ruzsinszky, G. I. Csonka, G. E. Scuseria, and J. P. Perdew, *Physical review letters* **111**, 106401 (2013).
- <sup>6</sup> R. Sabatini, T. Gorni, and S. de Gironcoli, *Phys. Rev. B* **87**, 041108 (2013).
- <sup>7</sup> O. A. Vydrov and T. Van Voorhis, *The Journal of Chemical Physics* **133**, 244103 (2010).
- <sup>8</sup> D. Mahlberg, S. Sakong, K. Forster-Tonigold, and A. Groß, *Journal of Chemical Theory and Computation* **15**, 3250 (2019), pMID: 30964999.
- <sup>9</sup> J. Wellendorff, T. L. Silbaugh, D. Garcia-Pintos, J. K. Nørskov, T. Bligaard, F. Studt, and C. T. Campbell, *Surface Science* **640**, 36 (2015).
- <sup>10</sup> J. Wellendorff, K. T. Lundgaard, A. Møgelhøj, V. Petzold, D. D. Landis, J. K. Nørskov, T. Bligaard, and K. W. Jacobsen, *Physical Review B* **85**, 235149 (2012).
- <sup>11</sup> H. Peng, Z.-H. Yang, J. P. Perdew, and J. Sun, *Phys. Rev. X* **6**, 041005 (2016).
- <sup>12</sup> A. J. Hensley, K. Ghale, C. Rieg, T. Dang, E. Anderst, F. Studt, C. T. Campbell, J.-S. McEwen, and Y. Xu, *The Journal of Physical Chemistry C* **121**, 4937 (2017).
- <sup>13</sup> G. Kresse and J. Hafner, *Phys. Rev. B* **49**, 14251 (1994).
- <sup>14</sup> G. Kresse and J. Furthmüller, *Phys. Rev. B* **54**, 11169 (1996).
- <sup>15</sup> G. Kresse and D. Joubert, *Phys. Rev. B* **59**, 1758 (1999).
